# Supplementary material for: Ultrafast imprinting of topologically protected magnetic textures via pulsed electrons
Source: arXiv:1706.08288 source file (2017-06-26)
Supplement: Supplementary file 1 [file schaeffer2017ultrafastimprinting_supp_mat.pdf]

# Supplementary Materials: Ultrafast imprinting of topologically protected magnetic textures via pulsed electrons

A. F. Schäffer[1], H. A. Dürr[2], J. Berakdar[1]

[1]*Institut für Physik, Martin-Luther-Universität Halle-Wittenberg, 06099 Halle (Saale), Germany and*

[2]*Stanford Institute for Materials and Energy Sciences, SLAC National Accelerator Laboratory, 2575 Sand Hill Road, Menlo Park, California 94025, USA*

(Dated: May 27, 2017)

## I. ELECTRON PULSE DRIVEN PRECESSIONAL SWITCHING OF FERROMAGNETIC FILMS

### A. Analytical Model

To substantiate both, the experimental and numerical results, a straightforward analytical ansatz is established. Here we model the system behavior using a mono-domain, macrospin picture in the presence of spatially structured magnetic field. The moment's dynamics is governed by the Landau-Lifshitz-Gilbert equation[2, 3]

$$\frac{d\mathbf{m}}{dt} = -\frac{\gamma}{1+\alpha^2}[\mathbf{m}\times\mathbf{B}(\mathbf{r},t)] - \frac{\alpha\gamma}{1+\alpha^2}[\mathbf{m}\times[\mathbf{m}\times\mathbf{B}(\mathbf{r},t)]] \tag{S1}$$

which captures the (low-energy) precessional and damped part of the spin motion. During the pulse we neglect the influence of the internal fields for simplicity. As we are dealing with only one single spin driven by the oersted-field of the electron bunch, we can simplify and separate the equations of motion for the components of $\mathbf{m}$. The generated magnetic fields of a classical electron-beam propagating in the $z$ direction has a $B_\varphi$ component only, as inferred from Biot-Savart's law in cylindrical coordinates. For the switching behavior, mainly the $z$ component of the magnetization is relevant. Therefore, the sign of $m_z$ after the pulse is in the focus of interest. The pulses temporal profile can, for example, be approximated by a $\sin^2$ envelope $B(t) = B_0 \sin^2(\frac{\sqrt{\pi}t}{2\delta})$ where $\delta$ denotes the pulses duration. The factor $\sqrt{\pi}/2$ is introduced for normalization reasons. The measured damping in the granular sample amounts a quite large value for the Gilbert damping-parameter $\alpha = 0.3$ the magnetization relaxes rapidly towards one of the two possible easy directions of anisotropy. The time-dependence of $m_z$ during the pulse can be deduced to be

$$m_z(t) = \cos\left[c_1 B_0 \left(t - \tilde{\delta}\sin(t/\tilde{\delta})\right)\right] / \cosh\left[\alpha c_1 B_0 \left(t - \tilde{\delta}\sin(t/\tilde{\delta})\right)\right] \ , \tag{S2}$$

with $\tilde{\delta} = \delta/\sqrt{2}$ and $c_1 = \frac{\gamma}{2(1+\alpha^2)}$ Following this result, one can compute $m_z$ at the end of the pulse as a function of the external field value. The value $m_z(\delta)$ depending on the pulse duration and the strength of the magnetic pulse is displayed in fig. S1. As expected an alternating pattern with decreasing amplitude can be seen. Examining an ideal parameter-regime in which a switching occurs reliably, the region around $(5\,\mathrm{T}, 2\,\mathrm{ps})$ seems to be preferable because of the broad dark area. This means that the spin flip takes place even if there are small fluctuations in the pulse duration or the magnetic field amplitude.

As the Oersted-fields decay typically as $\sim \rho^{-1}$, the experimental data can be reproduced by the calculations of the final spin-orientation for the spatially varying $B_0 = B_\varphi(\rho) = B_{\max}/(\rho+\epsilon)$. In this part of the presented work, the focus is set on extended systems with a size ranging in the order of several hundred microns. Therefore the calculations incorporate the pulse's far field only. In order to prevent the magnetic field from a divergent behavior at the origin, a small length $\epsilon = 20\,\text{nm}$ is added to the distance. In the far field this does not affect the results. Due to the radial symmetry the results can be extended by a rotation so that two-dimensional systems are modeled. The results are shown together with the numerical and experimental in the main text (Fig.1).

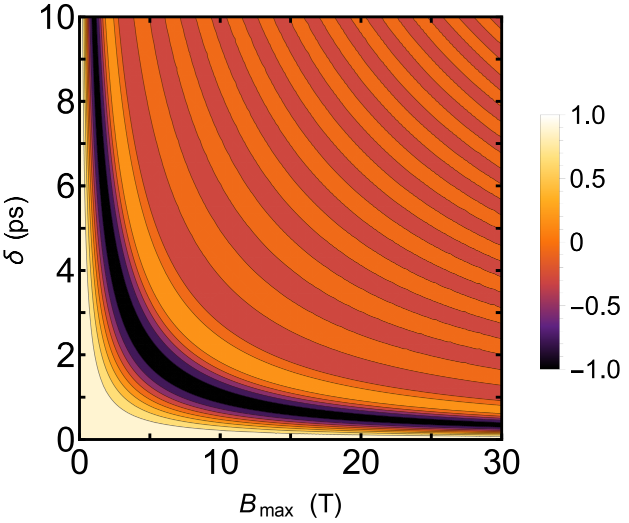


FIG. S1: Spin orientation after the magnetic pulse, depending on the amplitude $B_{\max}$ and the duration $\delta$.

## II. FULL NUMERICAL SIMULATIONS

In addition to the analytical approach, micromagnetic simulations are carried out. The material specific parameters are chosen to be equal to the measured ones ([1]), meaning a saturation magnetization $M_{\text{sat}} = 517.25\,\text{kA/m}$, the uniaxial anisotropy $K_{\text{u}} = 156.98\,\text{kJ/m}^3$ and the Gilbert damping parameter $\alpha = 0.3$.

Similar to the experimental work, we also consider a thin film of CoCrPt and a size of $150\,\mu\text{m}\times150\,\mu\text{m}\times14\,\text{nm}$. As the included Co-atoms lead to a granular structure, with

decoupled magnetic grains with a size of $20.6 \pm 4$ nm, we can model the system with discrete cells with a dimension of $(41.2 \times 41.2 \times 14)\,\mathrm{nm}^3$. To cover the desired area we need $3640^2$ cells.

In the described discretization, each simulation cell is associated with a magnetization $\mathbf{m}_i = \mathbf{M}_i/M_\mathrm{S}$ normalized to the saturation magnetization $M_\mathrm{S}$. The magnetization dynamics is governed by the Landau-Lifshitz-Gilbert equation [2, 3]

$$\dot{\mathbf{m}}_i = -\frac{\gamma}{1+\alpha^2}\left\{\mathbf{m}_i \times \mathbf{B}_i^{\mathrm{eff}}(t) + \alpha\left[\mathbf{m}_i \times \left(\mathbf{m}_i \times \mathbf{B}_i^{\mathrm{eff}}(t)\right)\right]\right\} \tag{S3}$$

where $\gamma = 1.76 \cdot 10^{11}$ 1/(Ts) denotes the gyromagnetic ratio and $\alpha$ is the dimensionless Gilbert damping parameter. The local effective magnetic field $\mathbf{B}_i^{\mathrm{eff}}(t)$ can be calculated following the equation $\mathbf{B}_i^{\mathrm{eff}}(t) = -1/M_\mathrm{S}\delta F/(\delta\mathbf{m}_i)$ and is therefore a functional of the system total free energy $F = F_\mathrm{EXCH} + F_\mathrm{MCA} + F_\mathrm{DMF} + F_\mathrm{ZMN}$. This quantity is influenced by the exchange interaction of adjacent magnetic moments $F_\mathrm{EXCH} = -A/c^2 \sum_{<ij>} \mathbf{m}_i \cdot \mathbf{m}_j$, the magnetocrystalline anisotropy $F_\mathrm{MCA}$, the demagnetizing fields $F_\mathrm{DMF}$, and the Zeeman-energy $F_\mathrm{ZMN}$. The MCA is typically uniaxial in nature for magnetic storage media, in the case of CoCrPt-alloys as well, with an easy axis in out-of-plane direction, which coincides with the cylindrical $z$-axis. Further details on the single contributions can be found for example in ref.[4]. In order to simulate the magnetization dynamics an adaptive Heun solver method has been used. As the excitation of the system takes place in a very short time scale the time step is fixed to 1 fs during the time evolution, which is calculated for an elapsed time of $300\,\delta$. Afterwards the new configuration is relaxed. This means that the precessional term of the LLG is disregarded for the purpose of a fast approach towards the final stable magnetic configuration.

Full GPU-based micromagnetic simulations using the simulation package `mumax3`[5] were employed to account for the effect of demagnetizing fields efficiently. Just like in the analytical approach, the electron beam is considered as a pulsed magnetic field in $\varphi$-direction, acting on the initially homogeneously magnetized ($\mathbf{m}_i = \hat{e}_z$) sample. To account for the influence of the DMF two results are shown in Fig.1(b,c) of the main text. The first neglects the DMFs and the second accounting for them. Both have in common that in a radius-range of about $10\,\mu$m a dark area similar to the experimental results arises, which signals a magnetization reversal in this region. The usual effect of the DMF favoring an in-plane magnetization can be seen but still the actual in-plane orientation should be investigated further, hence the

measurements could only unveil the $m_z$ component of the magnetic structure.

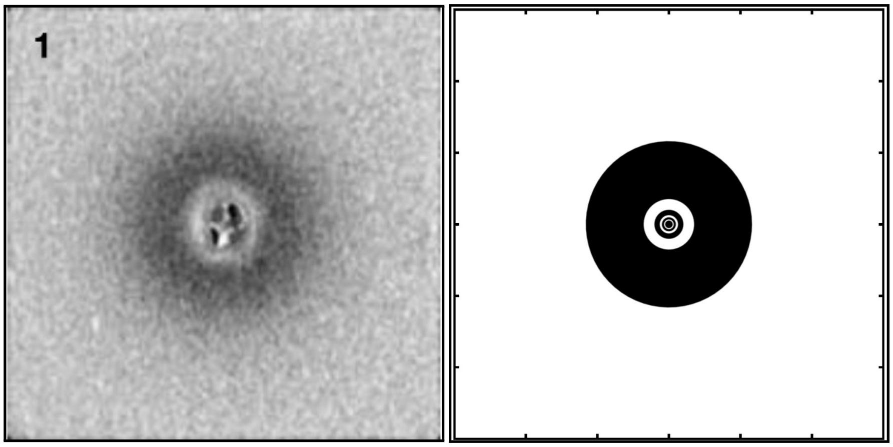


(a) (b)

FIG. S2: Comparison between experimental (a) and analytical (b) results. Figures correspond to an area of $150 \times 150\,\mu\text{m}^2$. The brightness stands for the $z$ component of the magnetization with white meaning $m_z = +\hat{e}_z$ and black $m_z = -\hat{e}_z$.

In the shown approaches the analytical and the numerical calculations are in line with each others and match well the experimental results. The simple analytical treatment neglects all kinds of effects arising due to collective phenomena. But already in this reduced picture, the ring-like domain-pattern can qualitatively be reproduced, taking into account the motion of a single spin, in the presence of the magnetic pulse. The large damping parameter was adapted from the previous works, which has been justified by arguments of spin fluctuations[1]. Nevertheless, the size of $\alpha$ does only affect the time needed by the system to relax towards either the spin up or down orientation. The sign of $m_z$ after the pulse is essentially dictated by the strength of the magnetic field and its duration.

## III. MAGNETIC NEAR FIELD

Up to now, only the magnetic far field of a localized electric current has been considered. For the investigated nano disc system the finite beam size becomes important, as it is

currently on the same size as the nanostructures. Therefore the calculation of the magnetic near field is indispensable. Here we assume again a pulse of electrons with a Gaussian envelope in space in time. The current density in cylindrical coordinates ($r$, $\varphi$ and $z$) reads as

$$j_z(r,\varphi,z) = \frac{N_e e v}{(2\pi)^{3/2}\sigma_{xy}^2\sigma_z} \exp\left[-\frac{1}{2}(r/\sigma_{xy})^2 - \frac{1}{2}((z-tv)/\sigma_z)^2\right] . \tag{S4}$$

Here $N_e$ corresponds to the number of electrons, $e$ is the electron charge, $v$ the average velocity and $\sigma_{xy}$ and $\sigma_z$ are the standard deviations in the related directions. The field's profile resulting from Biot-Savart's law

$$\mathbf{B}(\mathbf{r}) = \frac{\mu_0}{4\pi}\int_V \mathbf{j}(\mathbf{r}') \times \frac{\mathbf{r}-\mathbf{r}'}{|\mathbf{r}-\mathbf{r}'|^3}\mathrm{d}V' \tag{S5}$$

is shown in fig. S3 for two different sets of parameters. The curves shapes are almost the same, as in both cases the radial extension of the beam is much smaller than the standard deviation in the propagation direction. If this is changed the profiles do change as well. The peak field strength for the 30 $\mu$m beam is ten times smaller than the other pulse. This can be deduced from the number of electrons being a hundred times larger, but contrary the beam width is a thousand times wider, which leads to a resulting factor of 10.

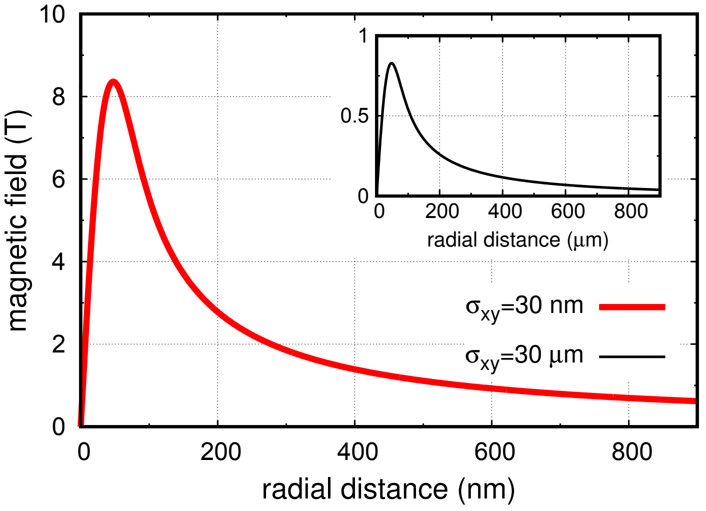


FIG. S3: Radial dependence of the peak magnetic field for a pulse duration of $\sigma_t = 2.3\,$ps. The red curve corresponds to $\sigma_{xy} = 30\,$nm and $N_e = 10^8$, whereas the black line relates to $\sigma_{xy} = 30\,\mu$m and $N_e = 10^{10}$.

[1] I. Tudosa, C. Stamm, A.B. Kashuba, F. King, H.C. Siegmann, J. Stöhr, G. Ju, B. Lu, and D. Weller, Nature **428**, 6985 (2004).

[2] L.D. Landau and E.M. Lifshitz, Phys. Z. Sowietunion **8**, 135 (1935).

[3] T.L. Gilbert, Physical Review **100**, 1243 (1955).

[4] A. Sukhov, P.P. Horley, J. Berakdar, A. Terwey, R. Meckenstock, and M. Farle, IEEE Transactions on Magnetics **50**, 12 (2014).

[5] A. Vansteenkiste, J. Leliaert, M. Dvornik, M. Helsen, F. Garcia-Sanchez, and B. Van Waeyenberge, AIP Advances **4**, 107133 (2014).
